# Supplementary material for: SIGL: Securing Software Installations Through Deep Graph Learning
Source: arXiv:2008.11533 source file (2021-06-22)
Supplement: Supplementary file 1 [file appendix.tex]

%\subsection{Detailed Comparison Results}
%\label{sec:details}
%\input{detailed_comparison}

\subsection{Major Revision Description}
We address all of the reviewer concerns in the major revision as follows:
\begin{itemize}[leftmargin=*]
	\setlength\itemsep{0em}
	
	\item We discuss (in~\autoref{sec:discussion}) and evaluate (in~\autoref{eval:results:adversarial}) adversarial scenarios 
	to demonstrate \system's robustness against attack evasion. We show that it is difficult to circumvent \system's detection
	approach. (Reviewer A, B \& C)
	
	\item We provide false positive (FP) percentage in~\autoref{table:eval:results:overall} and the absolute number of FPs
	we encountered in our enterprise in~\autoref{eval:results:comparison} and 
	in our experimental testbed in~\autoref{eval:results:linux} where additional experiments were performed. 
	We also discuss its implications in~\autoref{eval:results:comparison}. We show that the number of FPs is manageable.
	In fact, it is dramatically reduced compared to the commercial TDS used by the enterprise. 
	We also evaluated \system when it is trained on a diverse benign dataset in~\autoref{eval:results:meta} 
	and~\autoref{eval:results:linux}. (Reviewer A, D, \& E)
	
	\item We discuss how training data can be obtained in~\autoref{sec:discussion}.
	Additionally, we evaluate \system's robustness against data contamination in~\autoref{eval:results:contamination}. 
	Per reviewers' suggestions, we performed a controlled experiment where the training data is deliberately contaminated
	to understand the impact on detection performance. We show that \system is robust to data contamination.
	(Reviewer A \& B)
	
	\item We provide more details on how the installation graph is marked as anomalous in~\autoref{sec:framework:detection}. (Reviewer E)
	
	\item We evaluate \system's ability to build meta-models in~\autoref{eval:results:meta}.
	We show that \system maintains high detection performance with meta-models. (Reviewer D)
	
	\item We evaluate in~\autoref{eval:results:linux} \system's ability to detect malicious installers even when no malware binary is written to disk.
	We show that \system can detect malicious execution without malware creating any binary execution file. (Reviewer A \& E)
	
	\item We show in~\autoref{eval:results:linux} that \system does not need to build application-specific models to detect malicious installers;
	it can learn generalized benign installation behavior that is application-agnostic.
	We evaluate \system with a large variety of software and on different OS platforms and installation frameworks. (Reviewer C \& D)
	
	\item We provide more details on how node embeddings are constructed from directed random walk in~\autoref{sec:framework:embedding}. (Reviewer E)
	
\end{itemize}

\change{
%\subsection{Framework-Specific Meta-Model}
%\label{sec:appendix:meta}
%\input{framework_auc}
}
